# Supplementary material for: Computing Equilibria in Binary Networked Public Goods Games
Source: arXiv:1911.05788 source file (2022-04-01)
Supplement: Supplementary file 1 [file supplementary.tex]

\subsection{Pseudocodes for \texttt{Asynchronous-BR} and \texttt{Evolve}}
\balance
\begin{algorithm}[h]
	\caption{Asynchronous-BR}
	\begin{algorithmic}[1]
		\State \textbf{Input}: $\ActionVec$
		\For{$i=1, \ldots, n$}
		\If{$\Delta g_i(n_i) > c_i$}
		    \State $\Action{i} = 1$
		\ElsIf{$\Dg{i}{n_i} < c_i$}
		    \State $\Action{i} = 0$
		\Else
		    \State randomly set $\Action{i}=1$ or $0$ with probability $0.5$
		\EndIf
		\EndFor
	\end{algorithmic}
\end{algorithm}

\begin{algorithm}[h]
	\caption{Evolve}
	\begin{algorithmic}[1]
		\State \textbf{Input}: $\ActionVec, \numEvo$
		\State Initialize: $\epsilon^\ast=M, \ActionVec^\ast=\bm{0}$ \Comment{$M$: a large positive number}
		\For{$i=1, \ldots, \numEvo$}
		\State $\epsilon \leftarrow$ \Call{maxEpsilon}{$\bm{x}$} \Comment{\Call{maxEpsilon}{\ActionVec}: $\max\Set{U_i(1-\Action{i}, \InvNum{i}{\ActionVec}) - U_i( \Action{i}, \InvNum{i}{\ActionVec})}{i \in \V}$}
		\If{$\epsilon = 0$}
		    \State return \ActionVec \Comment{Find a PSNE}
		\EndIf
		\If{$\epsilon < \epsilon^\ast$}
		    \State $\epsilon^\ast = \epsilon, \ActionVec^\ast=\ActionVec$
		\EndIf
		\State $\bm{x} \leftarrow$ \texttt{Asynchronous-BR}($\bm{x}$)
		\EndFor
		\State return $\ActionVec^\ast$
	\end{algorithmic}
\end{algorithm}

% \subsection{Algorithm \texttt{TreePSNE}}
% \begin{algorithm}[H]
% 	\caption{TreePSNE}
% 		\begin{algorithmic}[1]
% 			\small
% 			\State \textbf{Input}: a BNPG game $(\mathcal{G}, \mathcal{U})$.
% 			\State \textbf{Initialize}: $T_R$
% 			\State Compute a Depth-first order $\mathcal{O}$ (start with leaves and end with the root)
% 			\For{$Y$ in $\mathcal{O}$ }
% 				\If{ $Y$ is the root}
% 					\State Compute $n_{R}^\prime$ conditioned on $x_R$.
% 					\State Compute the best responses of the root by a modified version of Algorithm 2.
% 				\ElsIf{ $Y$ is a leaf node}
% 					\State Compute the conditonal best-response table $T_Y$ by Algorithm 1.
% 					\State Pass $T_Y$ to its parent
% 				\Else{ $Y$ is an internal node}
% 					\State Compute the conditonal best-response table $T_Y$ by Algorithm 2.
% 					\State Pass $T_Y$ to its parent
% 				\EndIf
% 			\EndFor 
% 			\State Let $\hat{\mathcal{O}}$ be the reversed Depth-first order.
% 			\For{$Y$ in $\hat{\mathcal{O}}$}
% 				\If{ $Y$ is the root}
% 					\State Choose an action $x_R \in T_R$.
% 					\State Determine the actions of its children by the best-responses tables passed from them.
% 				\ElsIf{ $Y$ is a leaf node}
% 					\State Pass
% 				\Else{ $Y$ is an internal node}
% 					\State Determine the actions of its children by the best-responses tables passed from them.
% 				\EndIf
% 			\EndFor
% 			\State \textbf{Return}: A PSNE consists of the actions of the nodes. 
% 		\end{algorithmic}
% \end{algorithm}
